# Supplementary material for: FileBounty: Fair Data Exchange
Source: arXiv:2008.11362 source file (2021-07-09)
Supplement: Supplementary file 1 [file Appendix.tex]

\section{Appendix}

\subsection{Cryptographic Analysis}
\label{apx:cryptographicanalysis}
Once the seller $S$ starts serving $F$ with the deposit $D_S$ and, the buyer $B$ can choose to enter the contract with deposit $D_B$ and the file price $F_p$. Because $B$ and $S$ are aware of each other's public keys $Pub_B$ and $Pub_S$, they are able to use a key-exchange protocol in order to secure their non-blockchain based channel~\cite{canetti2001analysis} (i.e. a channel providing authenticity, integrity and confidentiality).% The buyer and seller separately connect to the blockchain and verify that the state of the smart contract is correct.

\subsubsection{File chunk integrity}
The buyer and seller then interact on the secure channel as follows: the seller sends $H_{k-1}^c$ and $c_k$ to the buyer, who verifies that $H_k^c = f(f(...f(H_{k-1}^c,M_{CL}^k)...),M_1^k)$. This guarantees the integrity of the chunk $c_k$, because we assume that it is computationally unfeasible for a polynomial-time adversary to find a preimage $x'$, given $y$ and $x$, such that $H(x') = y$ (i.e.\ second preimage resistance~\cite{al2010cryptographic}).

\subsubsection{Compromised Compression Function}
Depending on the file price, there may be an incentive for an adversary to find a second preimage of the underlying compression function. We distinguish between two cases: (i) the adversary pretends that the file is only one chunk long, and (ii) the adversary corrupts one chunk out of $n$ file chunks. Note that in the case where the adversary is capable of finding a second preimage, the smart contract won't be able to distinguish between a valid and invalid file chunk.
\begin{itemize}
\item \textbf{Crafted one chunk file}
An adversary could for instance, craft a chunk $c_1$, such that the length encoded in the chunk is smaller than the chunk size (e.g., 32 bytes), and the chunk's cryptographic hash matches $F(H)$. This behavior would only be rational if the cost of finding a second preimage is inferior to the file price, i.e.\ Equation~\ref{eq:nonformallysecure1} needs to hold for \name{} to be secure against a rational adversary.
\begin{equation}\label{eq:nonformallysecure1}
Cost_{\text{preimg}} \overset{\epsilon}{>} F_p
\end{equation}

\item \textbf{Corrupting one chunk in the file}
In some cases though, the adversary may possess the file $F$ and will want to substitute a file chunk with another specifically crafted file chunk for malicious purposes. 

By doing so, the adversary may gain a utility of $W(F)$ (because he is effectively corrupting the buyer's file), but needs to spend $ Cost_{\text{preimg}}$ to find a second-preimage of the file chunk. This misbehavior would only be rational, if the cost of finding a preimage is lower than the file price $F_P$ paid to the adversary plus his utility $W(F)$ derived from misbehaving (cf. Equation~\ref{eq:nonformallysecure2}). Therefore, our protocol is economically secure for compression functions whose cost of finding a collision is more than the total utility that the adversary can derive from misbehaving; otherwise, a formally secure cryptographic hash function is required.
\begin{equation}\label{eq:nonformallysecure2}
Cost_{\text{preimg}} \overset{\epsilon}{>} F_p + W(F)+F_c
\end{equation}
\end{itemize}
\subsubsection{Signed Acknowledgements}
Once the buyer has verified the integrity of the chunk $k$, the buyer signs the following message\footnote{Assuming the buyer does not buy the same file from the same seller twice, we do not require to add freshness to the signature through a nonce.}:
\begin{equation}\label{eq:Signed Acknowledgment Message k}
    A_k := Sign_{Priv_B}(label||H(F)||pad(k)||pad(Pub_S)))
\end{equation}

Note, that the buyer signs the acknowledgment of chunk $k$ with his private key $Priv_B$, which corresponds to a private key of an external Ethereum account. As such, this private key is capable of signing any transaction that originates from the corresponding public Ethereum address. To make sure that the signed message $A_k$ does not allow to trigger an arbitrary blockchain transaction, we prepend a constant label to the hash of the file (cf. Equation~\ref{eq:Signed Acknowledgment Message k}). Also, we pad the chunk number $k$ and the public key of the seller, $Pub_S$, to ensure that they have fixed lengths.

Once the seller receives $A_k$, he verifies its validity by decoding the signed message with the buyer's public key, $Pub_B$. Now, at any point, the seller may broadcast a transaction to the smart contract containing $A_k$. The smart contract verifies the buyer's signature and $A_k$ therefore acts as a non-repudiable acknowledgment from the buyer for the reception of file chunk $k$. %To this end, the smart contract is capable of verifying the signature of the buyer in $A_k$; note that, since the buyer signs the chunk number $k$, it is not possible for the buyer to repudiate the fact that he received a chunk.

\begin{table*}[!htb]\centering\small
\caption{Payout functions depending on the protocol state and the actions of the buyer and the seller. For each transition, the first row corresponds to the buyer and the second row to the seller payout. $T_k$ corresponds to the transmission of file chunk $k$. $A_k$ is the acknowledgement of file chunk $k$. Not acknowledging the chunk $k$ is denoted as $\overline{A_k}$. If the buyer does not report at chunk $k$ (i.e., $\overline{R^B_k}$), this is equivalent to not responding and being offline ($\bot^S$). $P_k$ signifies that the seller proves to own chunk $k$, while $\overline{P_k}$ means that the seller does not prove to own chunk $k$, which is equivalent to not responding and being offline. We denote by $\bot^S$ respectively $\bot^B$ to the timeouts by the seller, respectively the buyer.% The details of the cases where the buyer does not respond are given in Table~\ref{tab:payoutsdetails} (Appendix).
}\label{tab:payouts}
\begin{tabular}{lp{0.12\linewidth}p{0.13\linewidth}>{\raggedright\arraybackslash}p{0.34\linewidth}}
\toprule
Transition                                                                                                              & Smart Contract Payoff                                  & Utility Payoff                                     & Comment \\
\midrule
%(1)
$T_n \rightarrow A_n \rightarrow \dots \rightarrow T_{1} \rightarrow A_{1}$                                             & $D_B$ \par $D_S + F_p$                                 & $F_v$ \par $0$                                     & Final utility with honest behavior of buyer and honest behavior of seller \\
%(2)
% $T_k \rightarrow A_k \rightarrow \overline{T_{k-1}} \rightarrow R^B_{k-1} \rightarrow P_{k-1}$                          & $\frac{k}{n} \cdot F_p$ \par $\frac{n-k}{n} \cdot F_p$ & $g^B(n-k+1) \cdot F_v$ \par $g^S(n-k+1) \cdot F_c$ & Seller does not send chunk $k-1$, so buyer reports, yet seller proves \\
% %(3)
% $T_k \rightarrow A_k \rightarrow \overline{T_{k-1}} \rightarrow R^B_{k-1} \rightarrow \overline{P_{k-1}} \equiv \bot^S$ & $F_p + D_B$ \par $0$                                   & $g^B(n-k+1) \cdot F_v$ \par $g^S(n-k+1) \cdot F_c$ & Seller does not send chunk $k-1$ so buyer reports, then seller times out \\
% %(4)
% $T_k \rightarrow A_k \rightarrow \overline{T_{k-1}} \rightarrow %\overline{R^B_{k-1}} \equiv
% \bot^B$                     & $0$ \par $\frac{n-k}{n} \cdot F_p + D_S$               & $g^B(n-k+1) \cdot F_v$ \par $g^S(n-k+1) \cdot F_c$ & Seller does not send chunk $k-1$, but buyer is offline \\
%(5)
$T_k \rightarrow R^B_k \rightarrow P_k$                                                                                 & $\frac{k-1}{n} \cdot F_p$ \par $\frac{n-k+1}{n} \cdot F_p$ & $g^B(n-k+1) \cdot F_v$ \par $g^S(n-k+1) \cdot F_c$ & Seller sends chunk $c_k$, yet buyer reports; then seller proves \\
%(6)
$T_k \rightarrow R^B_k \rightarrow \overline{P_k} \equiv \bot^S$                                                        & $F_p + D_B$ \par $0$                                   & $g^B(n-k+1) \cdot F_v$ \par $g^S(n-k+1) \cdot F_c$ & Seller sends chunk $c_k$, yet buyer reports; then seller times out \\
%(7)
$T_k \rightarrow %\overline{R^B_k} \equiv
\bot^B$                                                                        & $0$ \par $\frac{n-k}{n} \cdot F_p + D_S$                     & $g^B(n-k+1) \cdot F_v$ \par $g^S(n-k+1) \cdot F_c$ & Seller sends chunk $c_k$, but buyer doesn't acknowledge and times out \\
%(8)
$\overline{T_k} \rightarrow R^B_k \rightarrow P_k$                                                                      & $\frac{k-1}{n} \cdot F_p$ \par $\frac{n-k+1}{n} \cdot F_p$ & $g^B(n-k) \cdot F_v$ \par $g^S(n-k) \cdot F_c$ & Seller does not send chunk $c_k$, then buyer reports and seller proves \\
%(9)
$\overline{T_k} \rightarrow R^B_k \rightarrow \overline{P_k} \equiv \bot^S$                                             & $F_p + D_B$ \par $0$                                   & $g^B(n-k) \cdot F_v$ \par $g^S(n-k) \cdot F_c$     & Seller does not send chunk $c_k$, then buyer reports and seller does not prove \\
%(11)
$\overline{T_k} \rightarrow \overline{R^B_k} \equiv \bot^B$                                                             & $0$ \par $\frac{n-k}{n} \cdot F_p + D_S$ \par          & $g^B(n-k) \cdot F_v$ \par $g^S(n-k) \cdot F_c$     & Seller does not send chunk $c_k$, yet buyer times out \\
%(10)
$\overline{T_k} \rightarrow A_k \rightarrow R^S_k \rightarrow \overline{P_k^B}\equiv\bot^B$                                                   & $0$ \par $D_S+D_B+F_p$                                 & $g^B(n-k)F_v$ \par $g^S(n-k)F_c$                   & Seller does not send chunk $c_k$, but the buyer acknowledges it anyway and gets punished for lying \\
$\overline{T_k} \rightarrow A_k \rightarrow R^S_k \rightarrow P^B_k$                                                   & $\frac{k}{n}\cdot F_P$ \par $\frac{n-k}{n}\cdot F_P$                                 & $g^B(n-k)F_v$ \par $g^S(n-k)F_c$                   & Seller does not send chunk $k$, but the buyer acknowledges it anyway and successfully proves \\
$\dots %\rightarrow \overline{R^B_k} 
\rightarrow \overline{R^S_k} \rightarrow WAIT$                                & N/A \par N/A                                           & $g^B(n-k+1) \cdot F_v$ \par $g^S(n-k+1) \cdot F_c$ & The transfer happened up until block k, yet neither buyer nor seller claim; the protocol waits for the first claim \\
\bottomrule
\end{tabular}
\end{table*}

\begin{figure*}[!htb]\centering
\includegraphics[width=0.8\textwidth]{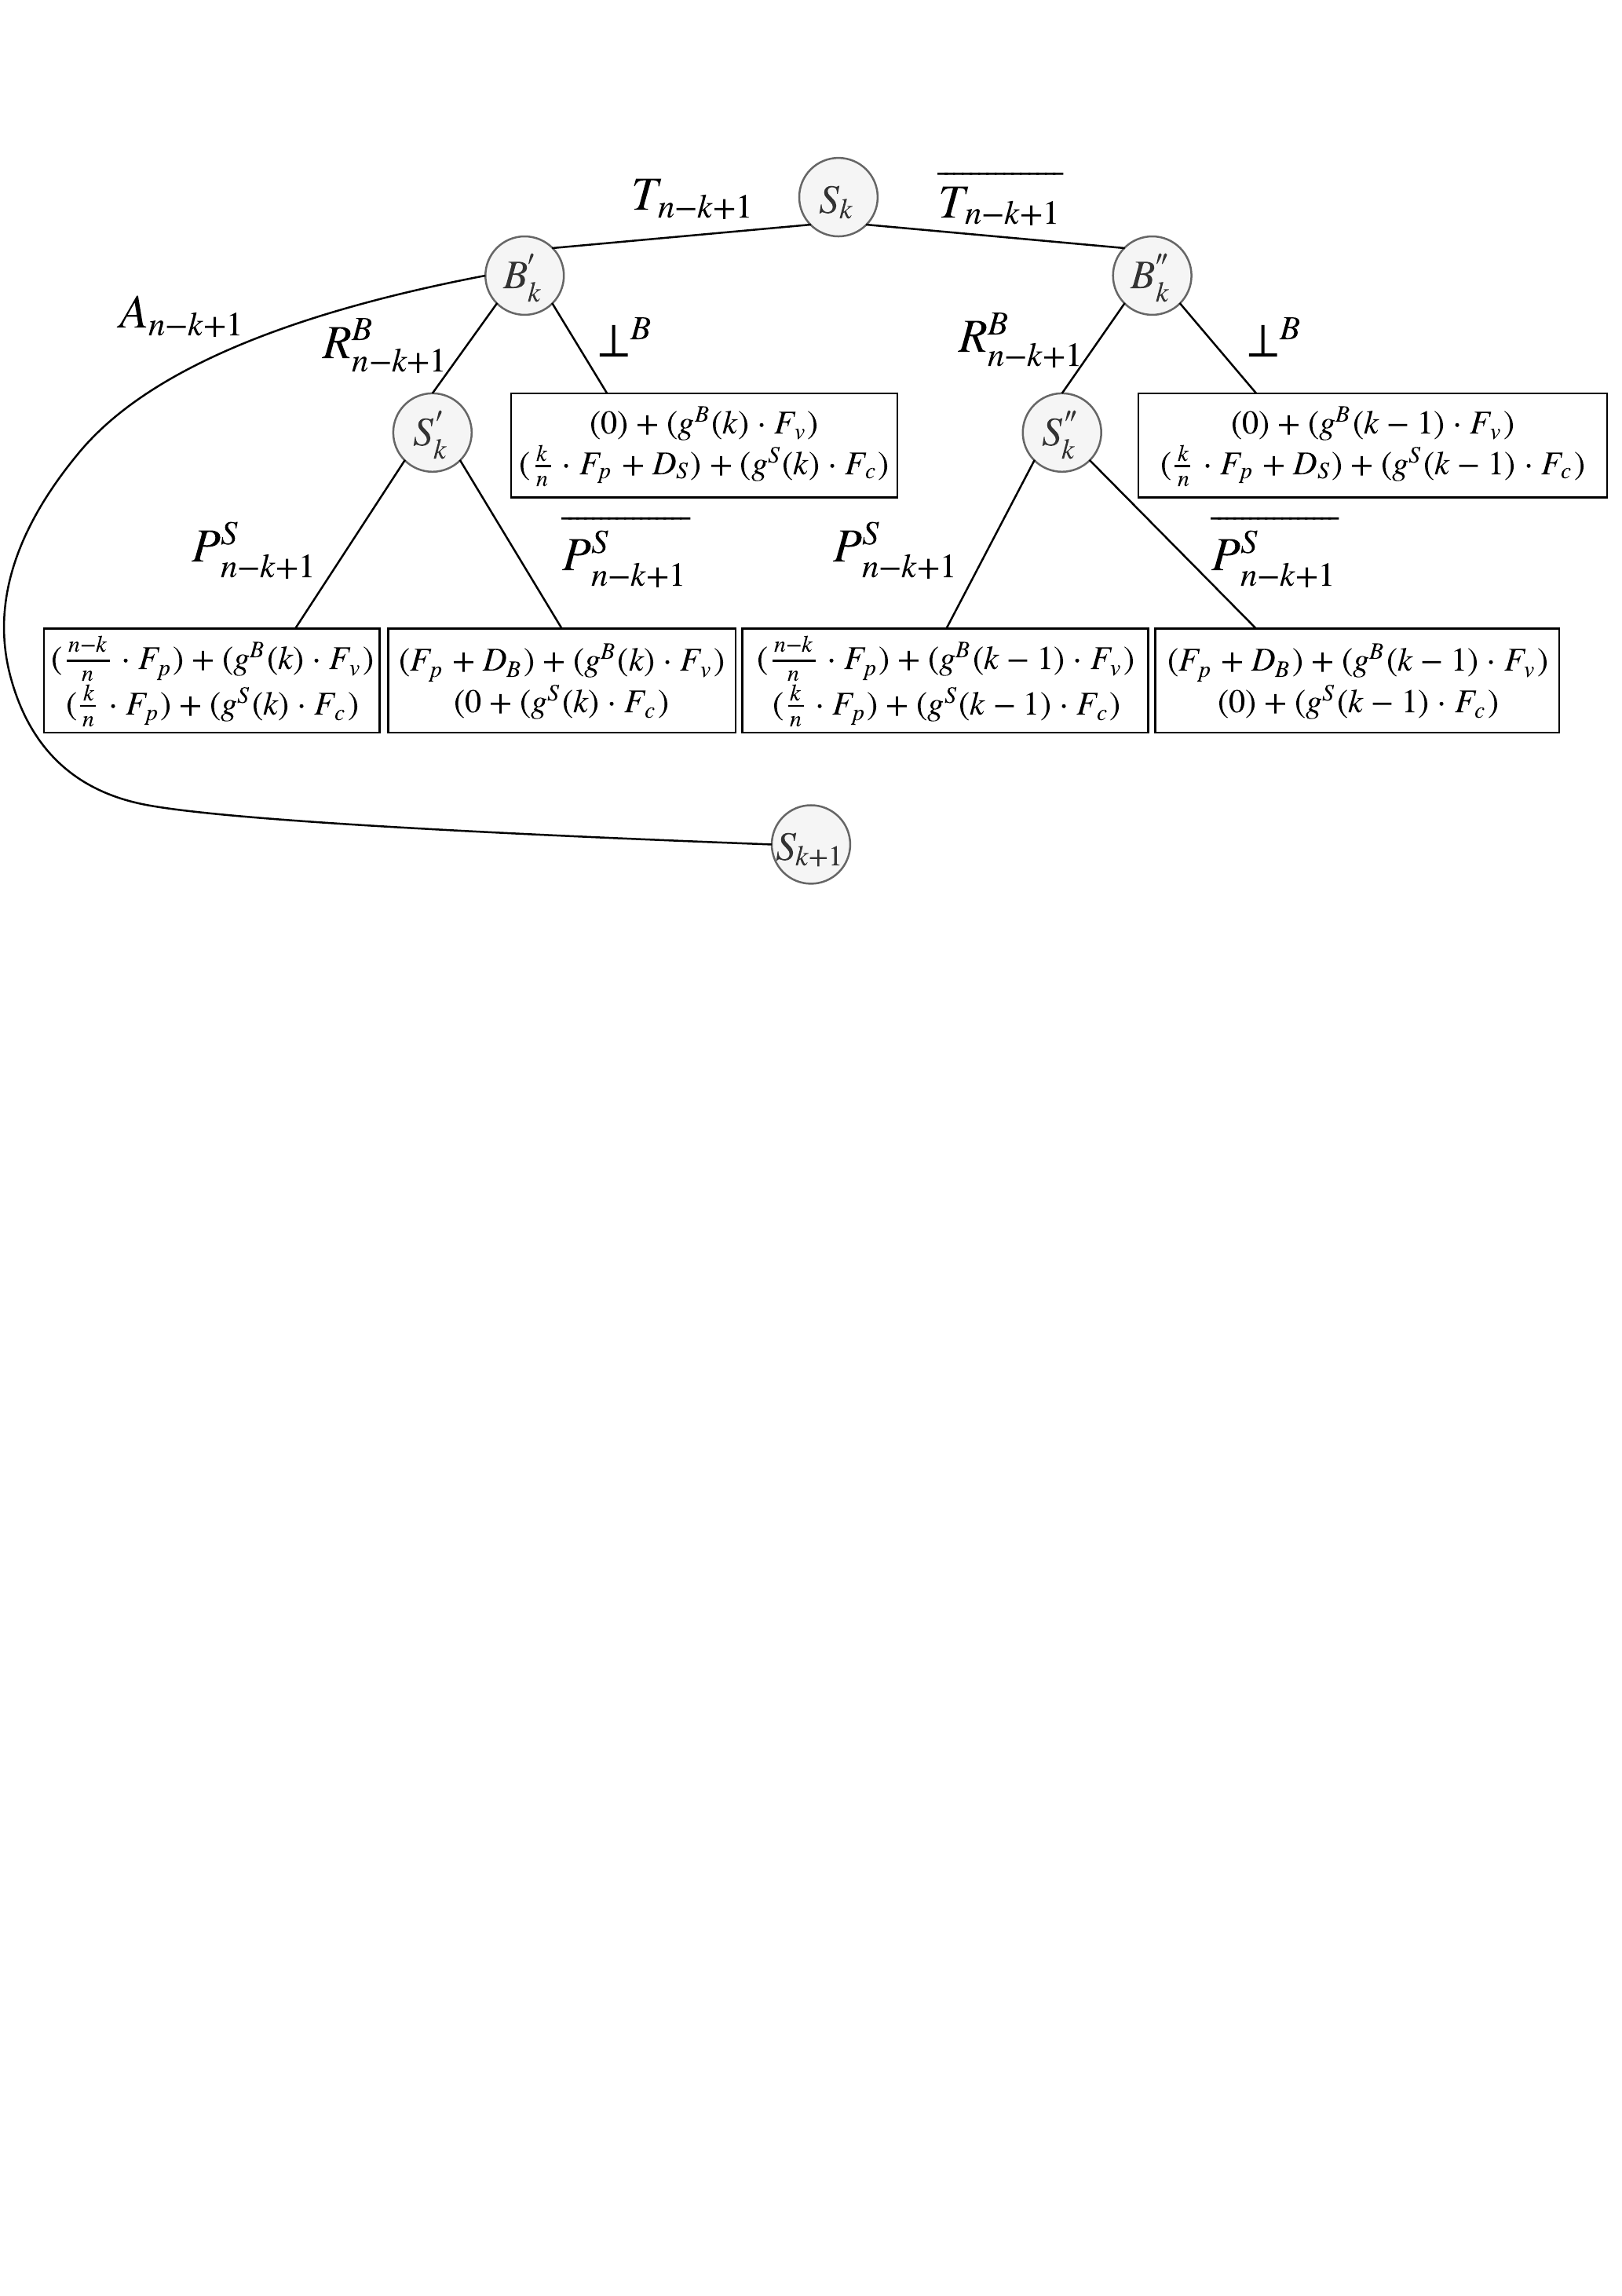}
\caption{Part of the game tree depicting strategies of both players when $k-1$ chunks are already transferred.}
\label{fig:subtree_k}
\end{figure*}

\subsection{Proof of Theorem~\ref{subgame_perfectness}}
\label{proof}
\begin{proof}
In Section~\ref{sec:attackanalysis}, we state that the buyer will never acknowledge a file chunk that hasn't been received, the reason being that acknowledging gives the seller the chance to claim the whole sum, and for the seller it is always strictly dominating strategy to do so. %On the other hand, this results in that the seller will never report the misbehavior of the buyer if he sends a correct file chunk to the buyer, because in this case he gets payoff $0$, strictly dominated strategy.
We disregard this part of the sequential game $G$ completely. This saves us from considering a game tree which consists of exponentially many states, so we instead deal with a tree of linear size.

Figure~\ref{fig:subtree_k} depicts the part of the extensive game tree in which $k-1$ chunks of the file are already transferred by the seller and acknowledged by the buyer. Node $S_k$ corresponds to the state in which it is the seller's turn to choose, send or not to send the $k$-th file chunk. 

We use backwards induction. The claim of the induction is that in each subtree rooted at $S_k$, honest behavior is the subgame perfect equilibrium, i.e. the seller sends chunk at each state and buyer acknowledges it. Final payments from the smart contract in case of honest behavior are $D_B$ for the buyer and $D_S+F_p$ for the seller. 

In the subtree rooted at the node $B_{k}''$, which corresponds to the state that the seller did not send the $k$-th chunk, buyer will always choose to report, $R_{n-k+1}^{B}$, and because of this the seller ends up with the utility 
$$\text{max}\{\frac{k}{n}F_p+g^S(k)F_c, g^S(k-1)F_c\}\leq \frac{k}{n}F_p+F_c,$$
on the other hand, the final utility for the seller in the honest behavior of both players  is equal to $F_p+D_S$, by backwards induction assumption. This implies that if $D_S$ is at least $F_p$ then $F_p+D_S\geq \frac{k}{n}F_p+F_c$, because the right-hand side is maximized when $k=n$ and we also know that $F_p\geq F_c$ by definition, otherwise the trade does not take place at all.

For the buyer an analogous argument works; in the state $B_{k}'$, where the seller already sent the $k$-th chunk, the buyer's payoff in case of playing $R_{n-k+1}^B$ is equal to $$\frac{n-k}{n}F_p+g^B(k)F_v,$$ while by the backwards induction hypothesis, if he plays $A_{n-k+1}$, his utility is equal to $D_B+F_v$. If we take $D_B\geq F_p$, then at each node $B_k'$, the buyer will play honestly, because $D_B+F_v\geq \frac{n-k}{n}F_p+g^B(k)F_v$ for any $k$. Therefore, the honest behavior corresponds to the subgame-perfect Nash equilibrium of the game $G$ with deposits of size $D_S=F_p$ and $D_B=F_p$. 

\end{proof}

%We provide in Table~\ref{tab:payoutsdetails} the remaining payout details (in particular what happens when one participant reports the other) and thereby extend the protocol specification of Table~\ref{tab:payouts}.

For the exposition purposes we did not consider all cases in the proof of the theorem. In fact those cases are treated analogously and the same result is derived.  
Note that the proof does not use any assumption on the relative utility functions $g^S(k)$ and $g^B(k)$. Improving on deposits is possible, at least for the given relative utility functions $g^S(k)$ and $g^B(k)$. The lower bounds obtained in the proof of theorem~\ref{subgame_perfectness} guarantee the honest behavior under any realizations of these functions.

{\color{blue}
\subsection{Smart Contract Implementation}\label{sec:appendiximplementation}
In the following, we describe the most significant functions that our \name{} smart contract implements.
\begin{description}
    \item[$setParametersAndPay()$] \strut \\ The seller sets up the smart contract parameters and sends the deposit $D_B$.
    \item[$acceptParametersAndPay()$] \strut \\ The buyer accepts the seller's conditions and pays the file price $F_p$ with the deposit $D_S$.
    % \item[setLastAppearance()] \strut \\ Every time a participant interacts with the smart contract, this function stores the timestamp of the last interaction for this specific participant. Participants can also call this function directly in order to avoid timeouts, as mentioned in the $report()$ function.
    % \item[confirmChunk()] \strut \\ The buyer acknowledged the seller's chunk $k$, the seller uses this function to set update the state and push the $MAX\_TIMEOUT$ limit. If the protocol was correctly executed, the seller calls this function just once with the buyer's acknowledgment in order to terminate the protocol and free the deposits.
    \item[$report()$] \strut \\ Can be called by both the buyer and the seller. The function challenges the other participant to prove he behaved correctly and sets a count down of $MAX\_TIMEOUT$, after which time he will be considered offline if he does not answer - after which the protocol comes to an end.
    \item[$prove()$] \strut \\ Can be called by both the buyer and the seller to settle a dispute. If needed, a block as well as a intermediate hash are taken as parameters so that the smart contract can verify that they hash to the correct value. The protocol then terminates and the payoffs are set accordingly.
    \item[$finalize()$] \strut \\ Once the protocol is over, seller can call this function in order to withdraw the payoffs of both sides.
\end{description}
}

\subsection{Related Work}\label{apx:relatedwork}
\begin{itemize}
\item \textbf{Fair Multiparty Computation}
Bentov et al.~\cite{bentov2014use} show how Bitcoin can be used to build fair multiparty protocols. A maliciously behaving party in particular will be forced to pay a predefined monetary penalty in case of misbehavior. The claim-or-refund functionality, is a building block of our contribution.

Andrychowicz et al.~\cite{andrychowicz2014fair} propose how to use Bitcoin to obtain fairness in any two-party secure computation protocol. While Andrychowicz et al.'s contribution is related to ours, and even explains how to use their scheme for the trade of digital goods, in our case however, the seller and buyer are not required to share any secret for the fair data exchange.
Andrychowicz et al.~\cite{andrychowicz2014secure} show how to use Bitcoin to perform multiparty computation using a version of ``timed commitments'', where the committer has to reveal his secret within a certain time frame, or to pay a fine. We make use of this principle in our work.

Similar to Andrychowicz et al.~\cite{andrychowicz2014fair}, Banasik et al.~\cite{banasik2016efficient} require the buyer to define a function which specifies the content of interest that the buyer would like to purchase. As such, their scheme can, for example, be used for the purchase of the factorization of RSA modulus. To apply their concept to the exchange of files with the use of zero-knowledge, their hash functions require specific properties that common hash functions (SHA1, SHA2, SHA3, etc.) do not possess.

Bao et al.~\cite{bao1999multi} show how to use a verifiable encryption scheme to do multiparty fair exchange where the trusted party can be offline. However, the third party needs to read the messages and contrary to our work, there is no deterministic way to check the integrity of the file. Kilinc et al.~\cite{kilincc2015optimally} extend on Bao's work regarding multiparty fair exchange, by maintaining the privacy of the messages exchanged.

Lysyanskaya et al.~\cite{lysyanskaya2006rationality} discuss rationality and adversarial behavior in the case of multiparty computations. This framework distinguishes rational and adversarial behaviors, where rational participants maximize the utility while adversaries behave arbitrarily.

\item \textbf{Multiparty Fair Exchange}
Franklin et al.~\cite{franklin1997fair} make the fundamental observation, that fair exchange is not useful if a document holder can substitute an arbitrary (and worthless) document for the one that is expected. Similar to Franklin et al. we assume that the buyer possesses a one-way hash of the file that it desires (or the one-way hash of an encryption of the file). Franklin et al. makes use a one-way function, that must have a group structure and the following equation to hold: $F(z,f(y)) = f(zy)$ -- which is not the case of the one-way hash functions used in practice.

Asokan et al.~\cite{asokan1998optimistic} provide a generic optimistic fair exchange by using a general topology and a TTP for the swap of exchangeable items.

Park et al.~\cite{park2003constructing} present a Fair-Exchange protocol via a distributed computation of RSA Signatures. The same year, Dodis et al.~\cite{dodis2003breaking} break the scheme and show how to modify it in order to achieve the same properties. Nonetheless, the integrity of the message (the file) is not guaranteed by those protocols. Zhou et al.~\cite{zhou2000some} summarize the state of fair exchange protocols research at the time (2000).

Kupccu and Lysyanskaya~\cite{kupccu2010usable} present another fair exchange protocol, but using e-cash. This work does not support an efficient way to verify that the file exchanged is the desired one (i.e. corresponds to the desired hash), which forces the authors to use a more restricted definition of fairness where they have to give the dishonest participant's deposit to the honest party in the case of dispute. We believe that this introduces undesirable game-theoretic incentives, as it gives an attacker a risk-free way to steal money from an honest participant. Since the integrity of each chunk is verified from the very beginning of our protocol, an attacker that does not possess the file will lose his deposit immediately without causing any risk to the buyer.

Garay et al.~\cite{garay2003timed} introduce a timed fair exchange protocol for digital signatures. If it were used for files like in our work, this protocol would not guarantee their integrity. Also, the generation of the zero-knowledge proofs is costly.

In our construction for \name{}, we make use of the gradual release paradigm as defined by Brickell et al.~\cite{brickell1987gradual}.

\item \textbf{Contract Signing}
Ateniese~\cite{ateniese1999efficient} presents an optimistic fair exchange protocol for digital signatures and contract signing. This does not cover the case of file exchange, as the message has to be known a priori. GauthierDickey and Ritzdorf~\cite{gauthierdickey2014secure} present a protocol for peer-to-peer games that enables players of the network to exchange game items. In their work, detection of cheating is probabilistic and the protocol relies on the assumption that enough players remain online. Bao et al.~\cite{bao1998efficient} propose a fair exchange protocol with an off-line TTP. One weakness of their protocol is that the off-line TTP must possess the file. They then show a verifiably committed signature scheme based on Gap-Diffie-Hellman groups, similar to Boldyreva~\cite{boldyreva2003threshold}.

\item \textbf{Proof of Ownership} Techniques of deduplication are often used in cloud storage providers in order to only store data once~\cite{halevi2011proofs}. Cryptographic hashes are one of the main building blocks to identify a file chunk that is being stored online. Similar to our work, proof of ownership suffers from possible attacks, where an adversary possesses only a fraction of a file, but claims to possess the entire file~\cite{di2012boosting}. Our protocol, however, makes sure that, assuming the security of the underlying compression function, an adversary cannot claim to possess a file, without owning the file.
\end{itemize}

% \subsection{}
% Ethereum can currently support around $500\,000$ on-chain transactions per day, which implies that the upper limit of \name is $250\,000$ downloads per day. 
